# Supplementary material for: Atomistic insights into hydrogen migration in IGZO from machine-learning interatomic potential: linking atomic diffusion to device performance
Source: arXiv:2508.19674 ancillary file (2025-08-27)
Supplement: Supplementary file 1 [file igzo_SI.pdf]

# Supporting Information

# Atomistic Insights into Hydrogen Migration in IGZO from Machine-Learning Interatomic Potential: Linking Atomic Diffusion to Device Performance

*Hyunsung Cho,*[a] *Minseok Moon,*[a] *Jaehoon Kim,*[a] *Eunkyung Koh,*[b] *Hyeon-Deuk Kim,*[b]

*Rokyeon Kim,*[b] *Gyehyun Park,*[b] *Seungwu Han,*[ac] *and Youngho Kang*[*d]

[a] Department of Materials Science and Engineering and Research Institute of Advanced Materials, Seoul National University, Seoul 08826, Republic of Korea.

[b] Display Research Center, Samsung Display Company Ltd., Yongin-si 17113, Republic of Korea.

[c] Korea Institute for Advanced Study, Seoul 02455, Republic of Korea.

[d] Department of Materials Science and Engineering, Incheon National University, Incheon 22012, Republic of Korea.

[*] Corresponding author: Prof. Youngho Kang

E-mail: youngho84@inu.ac.kr

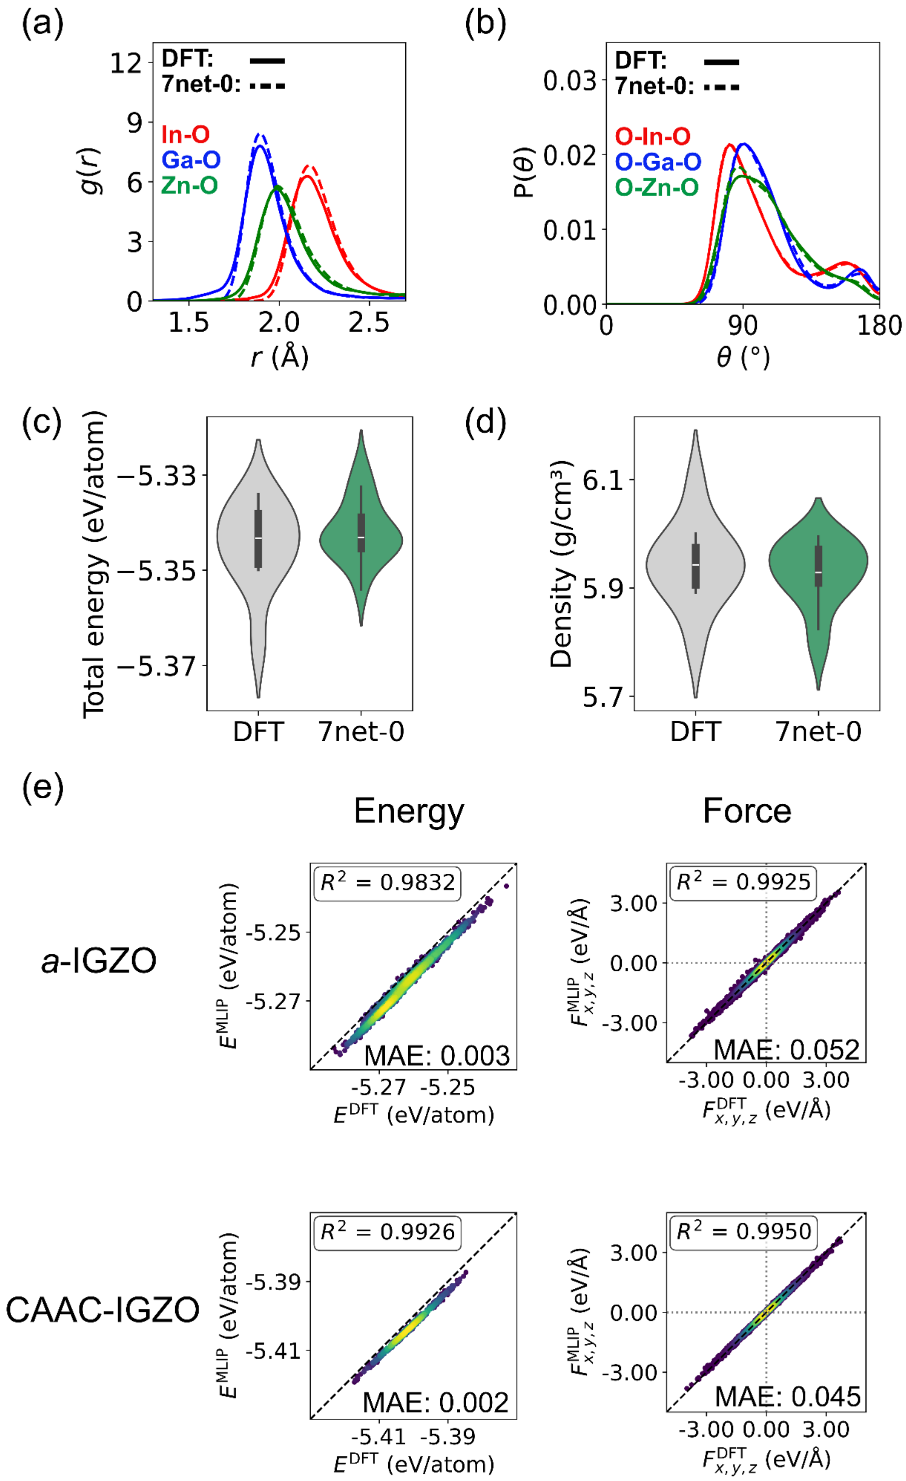


**Fig. S1.** Evaluation of prediction performance of pretrained 7net-0 model. (a) Radial distribution function (RDF), (b) angular distribution function (ADF), (c) total energy per atom, and (d) gravimetric density of pristine *a*-IGZO structures. (e) Energy and force parity plots for pristine *a*-IGZO and CAAC-IGZO systems. In (c) and (d), white dots indicate the median and black bars denote the interquartile range.

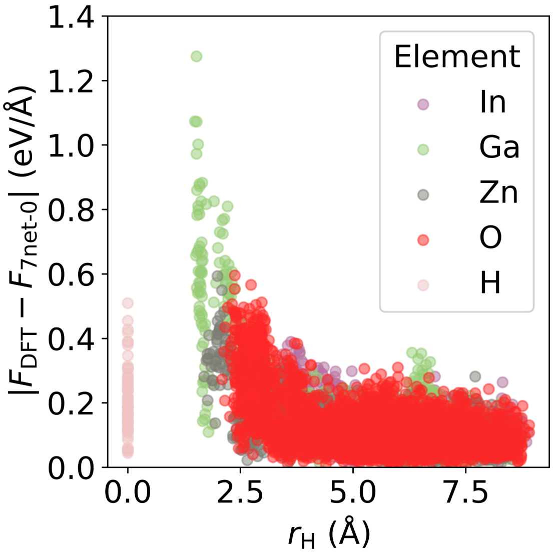


**Fig. S2.** Atomic force errors between DFT and 7net-0 as a function of distance from the substitutional hydrogen ($H_O$) defect along the 600 K annealing trajectory.

### Training dataset curation

The training set for the *a*-FT model consisted of 2,398 structures, primarily derived from 18-unit *a*-IGZO systems containing hydrogen-related defects. The dataset also included additional crystal In, Ga, and Zn oxide structures selected from the MPtraj dataset[1]. For the *a*-IGZO configurations, atomic structures were sampled from 600 K annealing and relaxation trajectories at regular intervals and subsequently re-evaluated using DFT one-shot calculations. DFT one-shot calculations for training set utilized a Monkhorst-Pack 3 × 3 × 3 *k*-point grid to improve accuracy. A subset of 360 structures from this dataset was set aside as a validation set.

The training set for the *c*-FT model was constructed by 800 CAAC-IGZO structures. Each CAAC-IGZO structure consists of a 16-unit (112-atom) configuration, with Ga and Zn atoms present in various combinations at the cation positions in the Ga/Zn-O layers. Interstitial hydrogen atoms were inserted into these configurations, and structures were sampled from MD trajectories annealed at 600 K and 1200 K, with 100 snapshots collected from each trajectory. DFT one-shot calculations for these crystal structure training set were performed using a Monkhorst-Pack 2 × 2 × 2 *k*-point grid. Out of the total 800 training structures used for the *c*-FT model, a subset of 200 structures was set aside as a validation set.

| System | | | Trajectory type | |
|---|---|---|---|---|
| **Target model** | **Reference** | **Created defect type** | **Relaxation** | **Annealing** |
| ***a*-FT** | Pristine | - | 144 (15 ens.) | 100 (5 ens.) |
| | Pristine | $H_O$ | 300 (30 ens.) | 300 (15 ens.) |
| | Pristine | $O{-}H_i$ | 150 (15 ens.) | - |
| | $O{-}H_i$ | $M{-}H_i$ | 150 (15 ens.) | - |
| | $O{-}H_i$ | $O{-}H_i$ | 150 (15 ens.) | - |
| | $O_{deficient}$ | - | 150 (15 ens.) | 100 (5 ens.) |
| | $O_{deficient}$ | $M{-}H_i$ | 250 (25 ens.) | - |
| | Crystal In-Ga-Zn-O based oxides in MPtraj[1] | - | 604 | - |
| ***c*-FT** | Pristine | - | - | 400 (2 ens.) |
| | Pristine | $O{-}H_i$ | - | 400 (4 ens.) |

**Table S1.** Training set composition. "*ens.*" means the number of ensembles. Defects are generated on the reference ensemble structures, followed by structural relaxation and annealing simulations.

**Fine-tuning procedure**

Fine-tuned models were developed from the pretrained 7net-0 model through full parameter tuning using continual learning, implemented via the SevenNet package[2]. The training procedure employed the Huber loss function, with a loss weight ratio of Energy:Force:Stress set to 1.00:1.00:0.01 ($\lambda_F = 1.00$ and $\lambda_S = 0.01$). Optimization was performed using the Adam optimizer, and the learning rate was scheduled via cosine annealing with warm-up. Each annealing cycle spanned 200 epochs, with the first 50 epochs designated for warm-up. The maximum and minimum learning rates were set to 0.001 and 0.0, respectively, and the training was carried out for a total of 600 epochs. The model checkpoint corresponding to the lowest validation error was selected as the final fine-tuned model.

$$\mathcal{L}_{\text{Huber}}(\hat{y}, y;\, \delta) = \begin{cases} \frac{1}{2}(\hat{y} - y)^2, & \text{for } |\hat{y} - y| \le \delta, \\ \delta\left(|\hat{y} - y| - \frac{\delta}{2}\right), & \text{otherwise.} \end{cases}$$

Huber loss function

$$\begin{aligned} \mathcal{L} = \frac{1}{M}\sum_{i=1}^{M} \mathcal{L}_{\text{Huber}}\left(\frac{\hat{E}_i}{N_i}, \frac{E_i}{N_i}, \delta\right) \\ + \lambda_F \frac{3}{M}\sum_{i=1}^{M} \frac{1}{N_i}\sum_{j=1}^{N_i}\sum_{k=1}^{3} \mathcal{L}_{\text{Huber}}(\hat{F}_{i,j,k}, F_{i,j,k}, \delta) \\ + \lambda_S \frac{6}{M}\sum_{i=1}^{M}\sum_{l=1}^{6} \mathcal{L}_{\text{Huber}}(\hat{S}_{i,l}, S_{i,l}, \delta). \end{aligned}$$

Total loss function of fine-tuned models

| MLIP model | Energy RMSE (meV/atom) | | Force RMSE (meV/Å) | | Stress RMSE (kbar) | |
|---|---|---|---|---|---|---|
| | Train | Valid | Train | Valid | Train | Valid |
| *a*-FT | 0.96 | 0.69 | 33.6 | 32.2 | 1.18 | 0.82 |
| *c*-FT | 0.10 | 0.14 | 17.6 | 18.5 | 0.31 | 0.35 |

**Table S2.** Training and validation root-mean-square errors (RMSE) for fine-tuning.

| System | O deficient | Pristine | O excessive | less H |
|---|---|---|---|---|
| [O defect] ($cm^{-3}$) | $1.0\times10^{20}$ | - | $1.0\times10^{20}$ | - |
| [H] ($cm^{-3}$) | $1.2\times10^{21}$ | $1.2\times10^{21}$ | $1.2\times10^{21}$ | $2.1\times10^{20}$ |
| $D_H$ ($cm^2s^{-1}$) | $1.65\times10^{-5}$ | $1.51\times10^{-5}$ | $1.22\times10^{-5}$ | $1.01\times10^{-5}$ |

**Table S3.** Hydrogen diffusivities in *a*-IGZO at various stoichiometry systems at 1300 K show that the diffusivity is essentially insensitive to changes in oxygen and hydrogen concentrations.

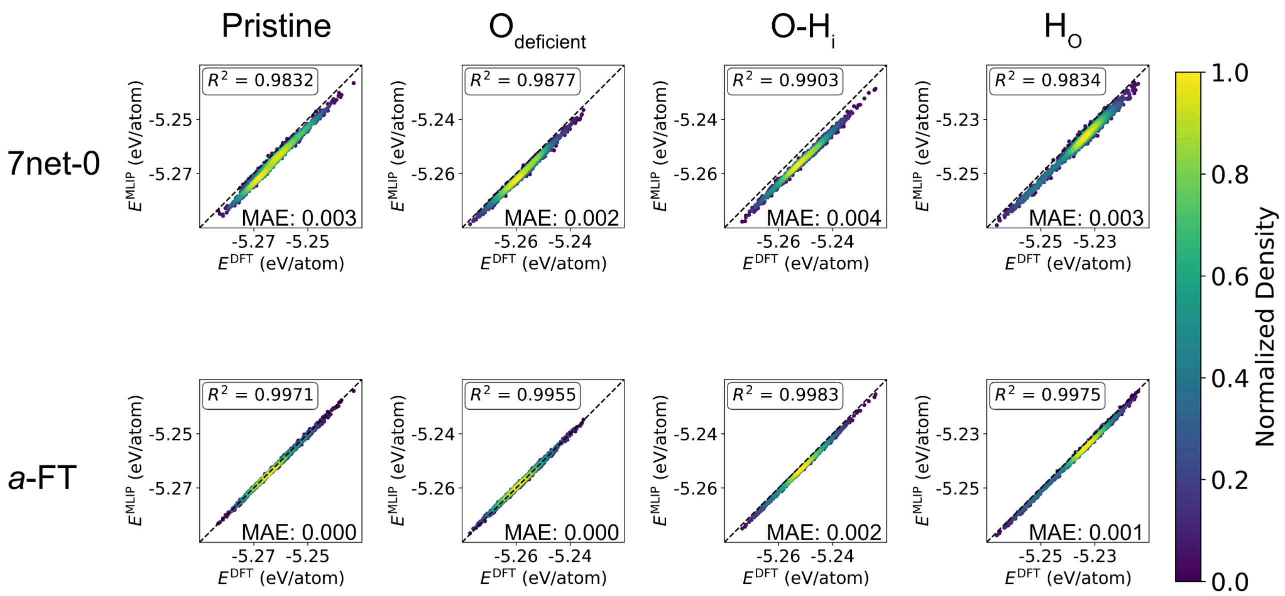


**Fig. S3.** Energy parity plots of *a*-IGZO systems for 600 K AIMD trajectories

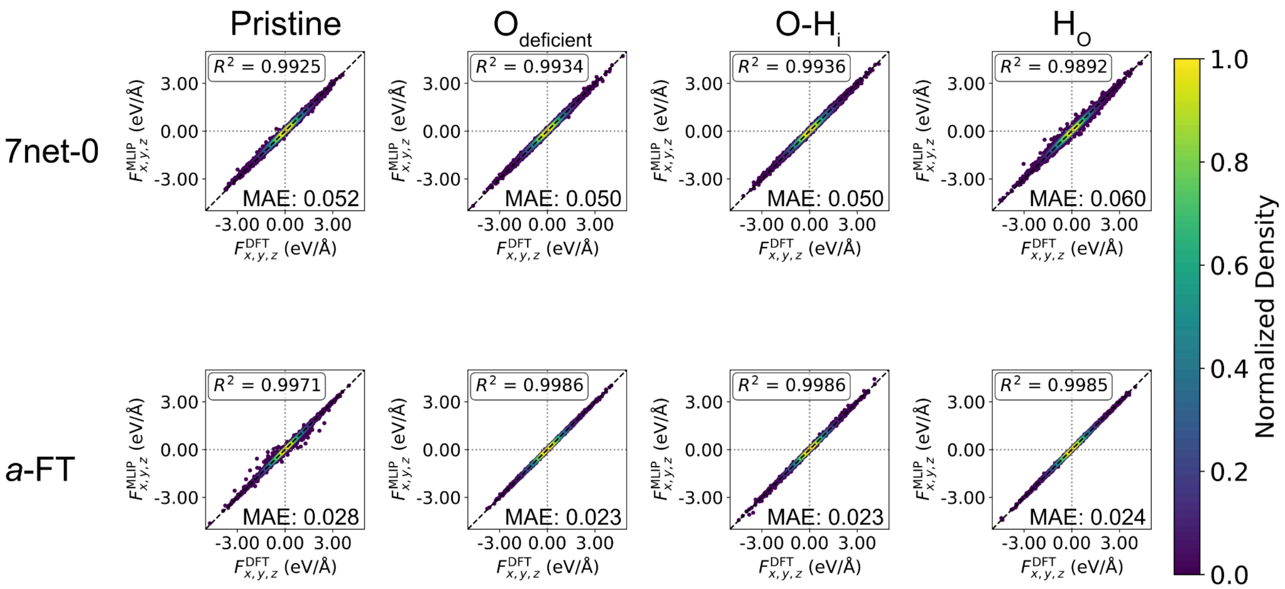


**Fig. S4.** Force parity plots of *a*-IGZO systems for 600 K AIMD trajectories

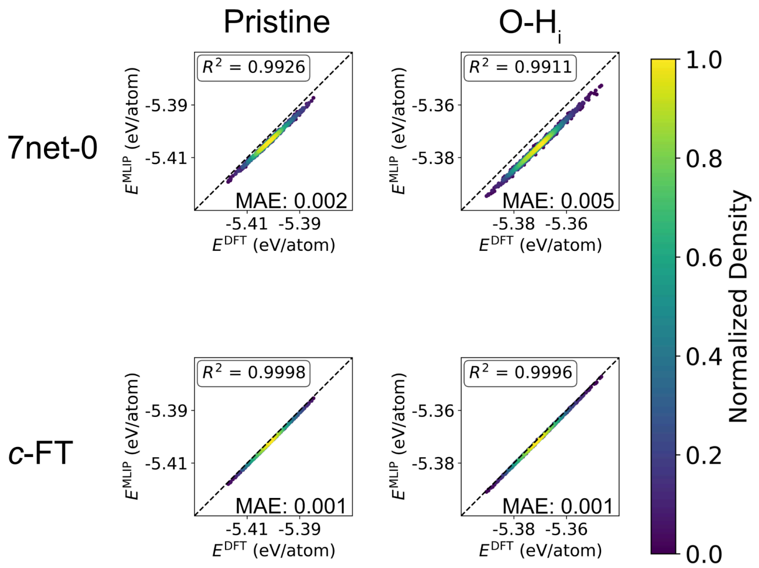


**Fig. S5.** Energy parity plots of CAAC-IGZO systems for 600 K AIMD trajectories

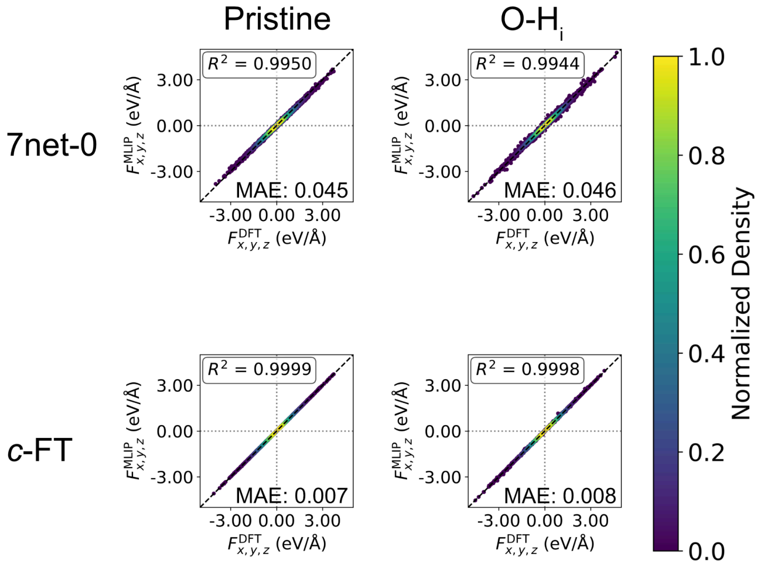


**Fig. S6.** Force parity plots of CAAC-IGZO systems for 600 K AIMD trajectories

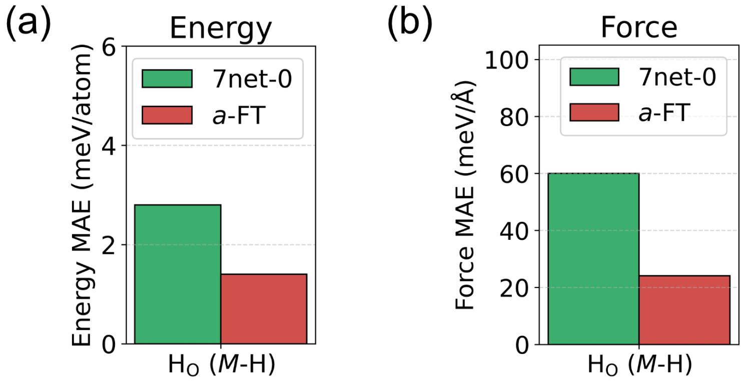


**Fig. S7.** (a) Energy mean absolute errors (MAEs) and (b) force MAEs for systems with $H_O$ forming *M*−H bonds.

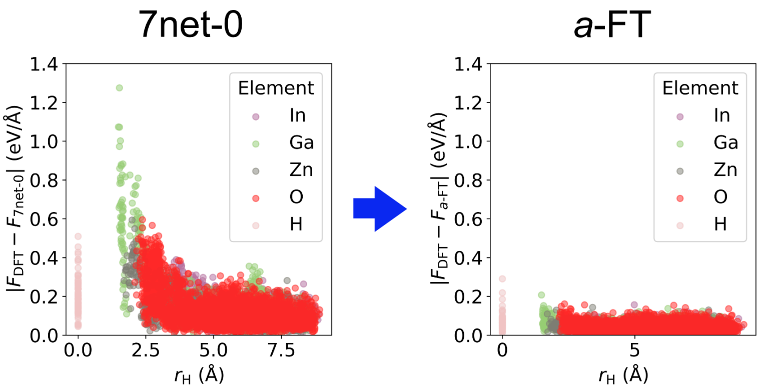


**Fig. S8.** Atomic force errors as a function of distance from the $H_O$ defect along the 600 K annealing trajectory. 7net-0 exhibits very large force errors on atoms close to $H_O$ and substantial errors throughout the entire simulation cell, whereas *a*-FT markedly suppresses these outliers, yielding a much more uniform and lower overall error.

**Relative energy ordering**

We evaluate relative energy ordering of three types of *M*-H defects, substitutional hydrogen $H_O$, $O_{def}$•*M*H, and $H_i$•*M*H. To construct the $O_{def}$•*M*H defect, an oxygen atom is removed prior to the melt-quench process during the preparation of the *a*-IGZO structure. In this case, oxygen removal leads to a delocalized electronic effect, with the system acting as a well-known $2e^-$ donor to conduction band[3,4]. When a $H_i$ is placed near a metal atom in this O-deficient structure, it can capture one of the conduction band electrons and form an *M*-H complex, referred to as $O_{def}$•*M*H. A similar mechanism applies to the $H_i$•*M*H defect. Since O-$H_i$ acts as a shallow donor, an additional hydrogen atom near a metal atom in the O-$H_i$-containing structure allows it to capture that electron and form another *M*-H complex. This defect configuration is denoted as $H_i$•*M*H.

For all types of *M*-H defects, 15 configurations are considered to capture structural diversity. As shown in Fig. S9, the *a*-FT MLIP model successfully reproduces the energy ordering for *M*-H defects, exhibiting strong linear correlation with DFT values.

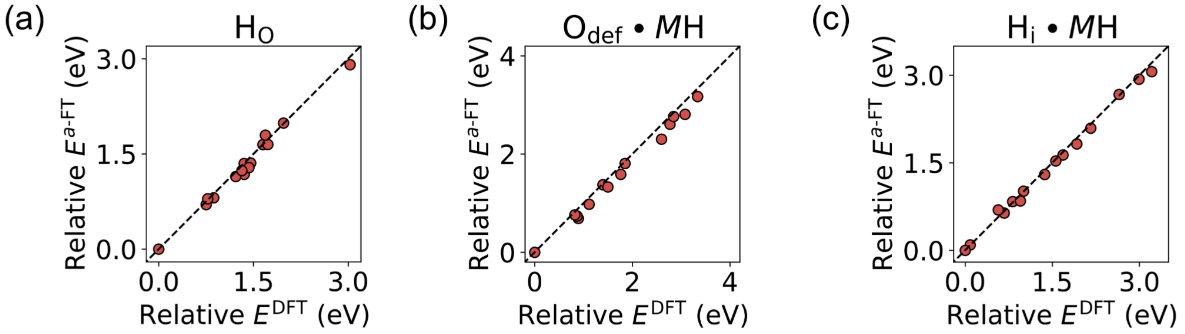


**Fig. S9.** Relative energies parity plots of *M*-H defects in *a*-IGZO between DFT and *a*-FT MLIP.

| $T$ (K) | 650 | 700 | 750 | 900 | 1050 | 1300 | 1700 |
|---|---|---|---|---|---|---|---|
| $D_H$ ($cm^2s^{-1}$) | $6.46\times10^{-9}$ | $3.20\times10^{-8}$ | $1.15\times10^{-7}$ | $6.88\times10^{-7}$ | $2.88\times10^{-6}$ | $1.51\times10^{-5}$ | $6.18\times10^{-5}$ |
| $D_0$ ($cm^2s^{-1}$) | $1.60\times10^{1}$ | | | $1.06\times10^{-2}$ | | | |
| $E_a$ (eV) | 1.21 | | | 0.74 | | | |

**Table S4.** Hydrogen diffusivity in *a*-IGZO at various temperatures. $D_H$ represents the temperature-dependent diffusivity of hydrogen, $D_0$ is the pre-factor obtained from Arrhenius relation fitting, and $E_a$ corresponds to the apparent activation energy.

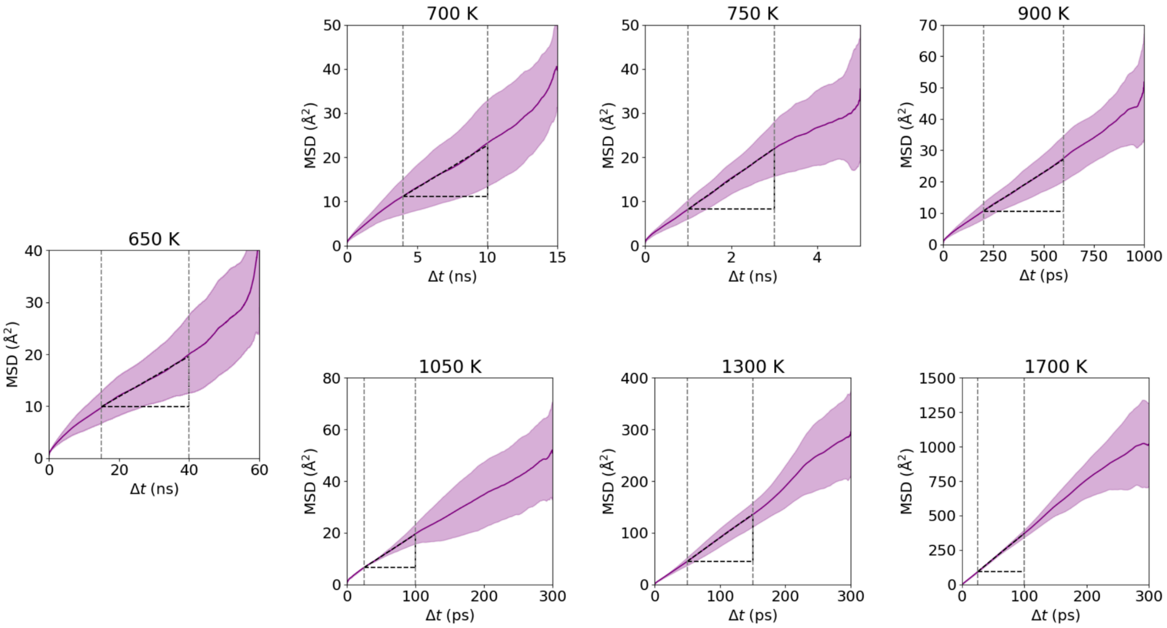


**Fig. S10.** Mean square displacement (MSD) of hydrogen atoms in *a*-IGZO as a function of time at various temperatures. Shaded regions represent the standard deviation. We select a narrow fitting region based on two criteria: (1) MSD values exceeding 10 Å² and (2) maximal linearity of the MSD curve. Extending the fitting window to include up to 60% of the maximum $\Delta t$ alters the results by less than 15%.

| $T$ (K) | 650 | 750 | 900 | 1000 | 1100 | 1300 | 1500 | 1700 |
|---|---|---|---|---|---|---|---|---|
| $D_H$ ($cm^2s^{-1}$) | $4.98\times10^{-7}$ | $8.93\times10^{-7}$ | $1.80\times10^{-6}$ | $2.00\times10^{-6}$ | $4.31\times10^{-6}$ | $1.01\times10^{-5}$ | $2.48\times10^{-5}$ | $3.67\times10^{-5}$ |
| $D_0$ ($cm^2s^{-1}$) | $3.25\times10^{-5}$ | | | | $2.19\times10^{-3}$ | | | |
| $E_a$ (eV) | 0.23 | | | | 0.59 | | | |

**Table S5.** Total hydrogen diffusivity in CAAC-IGZO at various temperatures. $D_H$ represents the temperature-dependent diffusivity of hydrogen, $D_0$ is the pre-factor obtained from Arrhenius relation fitting, and $E_a$ corresponds to the apparent activation energy.

| $T$ (K) | 650 | 750 | 900 | 1000 | 1100 | 1300 | 1500 | 1700 |
|---|---|---|---|---|---|---|---|---|
| $D_H$ ($cm^2s^{-1}$) | $6.84\times10^{-7}$ | $1.25\times10^{-6}$ | $2.35\times10^{-6}$ | $2.99\times10^{-6}$ | $6.42\times10^{-6}$ | $1.43\times10^{-5}$ | $3.42\times10^{-5}$ | $4.92\times10^{-5}$ |
| $D_0$ ($cm^2s^{-1}$) | $4.92\times10^{-5}$ | | | | $2.43\times10^{-3}$ | | | |
| $E_a$ (eV) | 0.24 | | | | 0.56 | | | |

**Table S6.** In-plane hydrogen diffusivity in CAAC-IGZO at various temperatures. $D_H$ represents the temperature-dependent diffusivity of hydrogen, $D_0$ is the pre-factor obtained from Arrhenius relation fitting, and $E_a$ corresponds to the apparent activation energy.

| $T$ (K) | 1300 | 1500 | 1700 |
|---|---|---|---|
| $D_H$ ($cm^2s^{-1}$) | $7.42\times10^{-7}$ | $3.07\times10^{-6}$ | $7.54\times10^{-6}$ |
| $D_0$ ($cm^2s^{-1}$) | $1.52\times10^{-2}$ | | |
| $E_a$ (eV) | 1.11 | | |

**Table S7.** Out-of-plane hydrogen diffusivity in CAAC-IGZO at various temperatures. $D_H$ represents the temperature-dependent diffusivity of hydrogen, $D_0$ is the pre-factor obtained from Arrhenius relation fitting, and $E_a$ corresponds to the apparent activation energy.

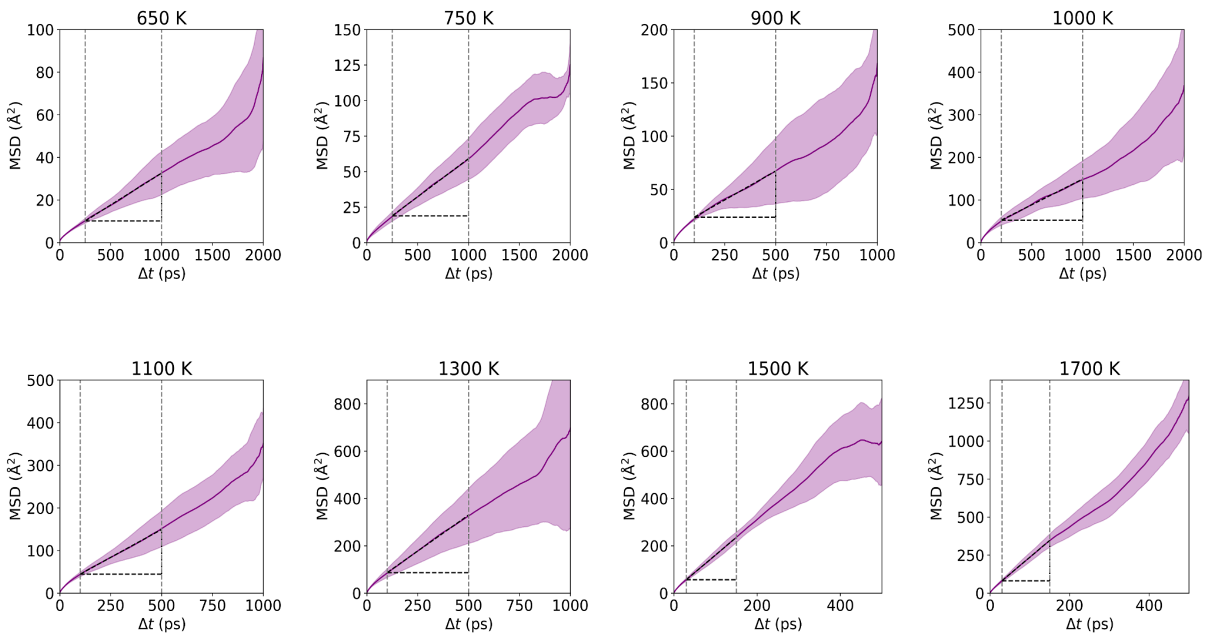


**Fig. S11.** Mean square displacement (MSD) of hydrogen atoms in CAAC-IGZO as a function of time at various temperatures. Shaded regions represent the standard deviation. We select a narrow fitting region based on two criteria: (1) MSD values exceeding 10 Å² and (2) maximal linearity of the MSD curve. Extending the fitting window to include up to 60% of the maximum $\Delta t$ alters the results by less than 15%.

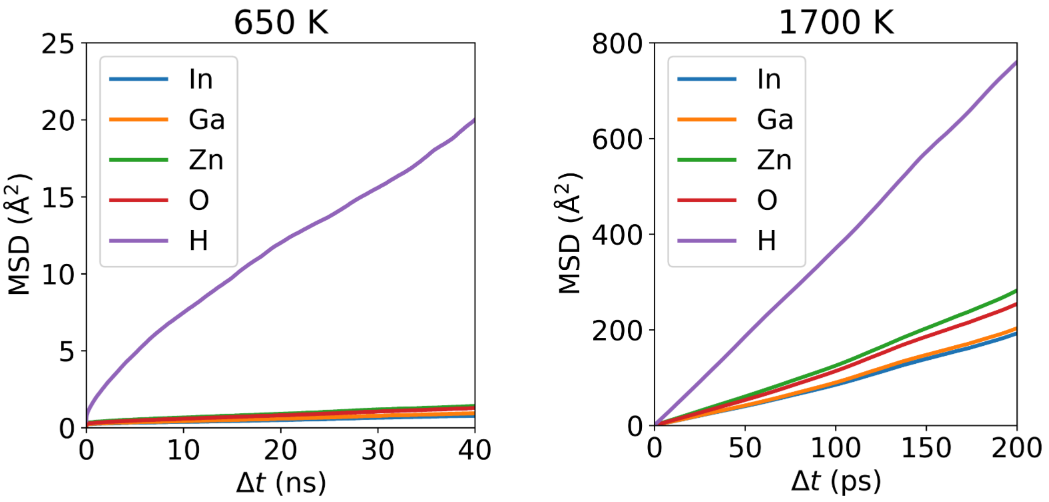


**Fig. S12.** Elementwise MSD plot for 650 K and 1700 K. At 650 K, cations and oxygen atoms primarily exhibit vibrational motion around their original positions, without significant long-range diffusion observed.

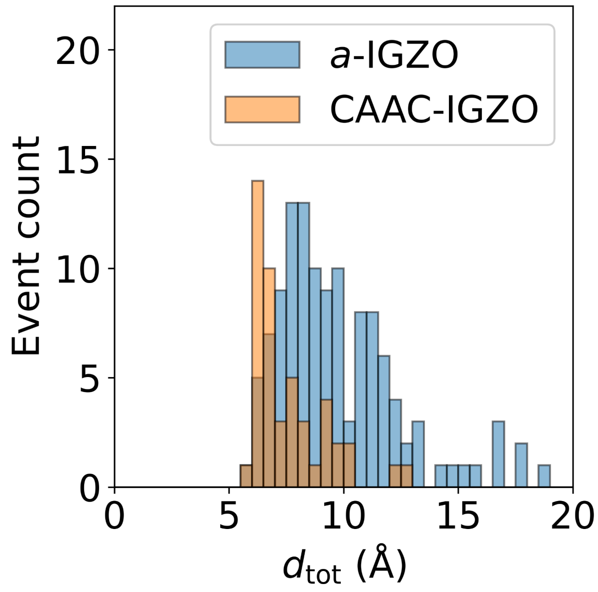


**Fig. S13.** Distribution of the total atomic displacements ($d_{tot}$) between initial state (IS) and transition state (TS) along the NEB paths. For *a*-IGZO, 121 ring-to-ring flipping (RTRF) events are sampled, while for CAAC-IGZO, 47 In-O layer penetration (IO-P) events are sampled as representative out-of-diffusion processes. The average $d_{tot}$ is 9.75 Å for RTRF and 7.58 Å for IO-P, indicating that *a*-IGZO exhibits more extended collective atomic motions than CAAC-IGZO during out-of-plane diffusion. The total atomic displacement is calculated as

$$d_{\mathrm{tot}} = \sum_{i=1}^{N} d_i = \sum_{i=1}^{N} \left\| \mathbf{R}_i^{(\mathrm{TS})} - \mathbf{R}_i^{(\mathrm{IS})} \right\|,$$

where $d_i$ is the displacement of atom $i$, $N$ is the total number of atoms, and **R** denotes the atomic position.

References

1 B. Deng, P. Zhong, K. Jun, J. Riebesell, K. Han, C. J. Bartel and G. Ceder, *Nat. Mach. Intell.*, 2023, **5**, 1031–1041.

2 Y. Park, J. Kim, S. Hwang and S. Han, *J. Chem. Theory Comput.*, 2024, **20**, 4857–4868.

3 T. Kamiya, K. Nomura, M. Hirano and H. Hosono, *Phys. Status Solidi C*, 2008, **5**, 3098–3100.

4 H. Song, G. Kang, Y. Kang and S. Han, *Phys. Status Solidi B*, 2019, **256**, 1800486
